# Supplementary material for: Task-agnostic Exploration in Reinforcement Learning
Source: arXiv:2006.09497 source file (2020-06-16)
Supplement: Supplementary file 1 [file appendix.pdf]

# Appendices

## A Proof of Upper Bound

In the proofs below we drop the superscript  $(n)$  for simplicity.

**Proof of Lemma 2.** Similar to Lemma 4.2 of [Jin et al., 2018], we can write down a recursive formula for both  $(Q_h^k - Q_h^{\pi_k})(s, a)$  and  $(\bar{Q}_h^k - \bar{Q}_h^{\pi_k})(s, a)$ , and perform a subtraction, which gives

$$[(\bar{Q}_h^k - \bar{Q}_h^{\pi_k}) - (Q_h^k - Q_h^{\pi_k})](s, a) \quad (8)$$

$$= \alpha_t^0 (Q_h^{\pi_k} - \bar{Q}_h^{\pi_k})(s, a) \quad (9)$$

$$+ \sum_{i=1}^t \alpha_t^i \left[ (\bar{V}_{h+1}^{k_i} - \bar{V}_{h+1}^{\pi_{k_i}}) - (V_{h+1}^{k_i} - V_{h+1}^{\pi_{k_i}}) \right] (s_{h+1}^{k_i}) \quad (10)$$

$$+ \sum_{i=1}^t \alpha_t^i \left[ [\hat{\mathbb{P}}^{k_i} - \mathbb{P}_h][\bar{V}_{h+1}^{\pi_{k_i}} - V_{h+1}^{\pi_{k_i}}](s, a) + (r_h^{k_i} - \mathbf{E}[r_h](s_h^{k_i}, s_h^{k_i})) \right] \quad (11)$$

$$+ \sum_{i=1}^t \alpha_t^i b_i. \quad (12)$$

We now show that  $[(\bar{Q}_h^k - \bar{Q}_h^{\pi_k}) - (Q_h^k - Q_h^{\pi_k})](s, a) \geq 0$  by induction on  $h = H, H-1, \dots, 1$  and  $k = 1, \dots, K$ . It is easy to see that the first term of right-hand side  $\alpha_t^0 (Q_h^{\pi_k} - \bar{Q}_h^{\pi_k})(s, a) \geq 0$  since  $\bar{Q}_h^{\pi_k} = 0$ . For the second term, consider two cases:

(1) If  $\max_a \bar{Q}_{h+1}^{k_i}(s_{h+1}^{k_i}, a) \geq H$ , then  $[(\bar{V}_{h+1}^{k_i} - \bar{V}_{h+1}^{\pi_{k_i}}) - (V_{h+1}^{k_i} - V_{h+1}^{\pi_{k_i}})](s_{h+1}^{k_i}) = H - (V_{h+1}^{k_i} - V_{h+1}^{\pi_{k_i}})(s_{h+1}^{k_i}) \geq 0$ .

(2) If  $\max_a \bar{Q}_{h+1}^{k_i}(s_{h+1}^{k_i}, a) < H$ , then

$$(\bar{V}_{h+1}^{k_i} - \bar{V}_{h+1}^{\pi_{k_i}})(s_{h+1}^{k_i}) = \max_a \left[ \bar{Q}_{h+1}^{k_i}(s_{h+1}^{k_i}, a) - \bar{Q}_{h+1}^{\pi_{k_i}}(s_{h+1}^{k_i}, a) \right] \quad (13)$$

$$\geq \max_a \left[ Q_{h+1}^{k_i}(s_{h+1}^{k_i}, a) - Q_{h+1}^{\pi_{k_i}}(s_{h+1}^{k_i}, a) \right] \quad (14)$$

$$\geq Q_{h+1}^{k_i}(s_{h+1}^{k_i}, \pi_{k_i}(s_{h+1}^{k_i})) - Q_{h+1}^{\pi_{k_i}}(s_{h+1}^{k_i}, \pi_{k_i}(s_{h+1}^{k_i})) \quad (15)$$

$$= (V_{h+1}^{k_i} - V_{h+1}^{\pi_{k_i}})(s_{h+1}^{k_i}) \quad (16)$$

where the first inequality is by the induction hypothesis.

Similar to the proof of Lemma 4.3 in [Jin et al., 2018], observe that  $(\mathbb{1}[k_i \leq K] \cdot [\hat{\mathbb{P}}^{k_i} - \mathbb{P}_h][\bar{V}_{h+1}^{\pi_{k_i}} - V_{h+1}^{\pi_{k_i}}](s, a) + (r_h^{k_i} - \mathbf{E}[r_h](s_h^{k_i}, s_h^{k_i})))_{i=1}^\tau$  is a martingale difference sequence. By Azuma-Hoeffding, we have that with probability  $1 - p/(SAHN)$ :

$$\begin{aligned} \forall \tau \in [K], \left| \sum_{i=1}^\tau \alpha_\tau^i (\mathbb{1}[k_i \leq K] \cdot [\hat{\mathbb{P}}^{k_i} - \mathbb{P}_h][\bar{V}_{h+1}^{\pi_{k_i}} - V_{h+1}^{\pi_{k_i}}](s, a) + (r_h^{k_i} - \mathbf{E}[r_h](s_h^{k_i}, s_h^{k_i}))) \right| \\ \leq \frac{c'(H+1)}{2} \sqrt{\sum_{i=1}^\tau (\alpha_\tau^i)^2 \cdot (\log N + \iota)} \leq c \sqrt{\frac{H^3(\log N + \iota)}{\tau}}, \end{aligned}$$

for some absolute constant  $c$ . Using a union bound, we see that with at least probability  $1 - p$ , the following holds simultaneously for all  $(s, a, h, k, n) \in S \times A \times [H] \times [K] \times [N]$ :

$$\left| \sum_{i=1}^t \alpha_t^i (\mathbb{1}[k_i \leq K] \cdot [\hat{\mathbb{P}}^{k_i} - \mathbb{P}_h][\bar{V}_{h+1}^{\pi_{k_i}} - V_{h+1}^{\pi_{k_i}}](s, a)) \right| \leq c \sqrt{\frac{H^3(\log N + \iota)}{t}} \quad (17)$$

424 Finally, since we choose  $b_t = c\sqrt{\frac{H^3(\log N + \iota)}{t}}$ , we have that the last two terms of  $[(\bar{Q}_h^k - \bar{Q}_h^{\pi_k}) -$   
 425  $(Q_h^k - Q_h^{\pi_k})](s, a)$  also adds up at least zero. Putting everything together, we have shown that  
 426 with probability at least  $1 - p$ ,  $[(\bar{Q}_h^k - \bar{Q}_h^{\pi_k}) - (Q_h^k - Q_h^{\pi_k})](s, a) > 0$  for all  $(s, a, h, k, n) \in$   
 427  $S \times A \times [H] \times [K] \times [N]$ . This concludes the proof. ■

428 Given Lemma 2, the proof of Theorem 1 follows from the proof sketch in the main text.

## 429 B Proof of Additional Properties of UCBZERO

430 We first give two lemmas:

431 **Lemma 7.** *For any  $(s, a, h, k) \in S \times A \times [H] \times [K]$ , let  $t = N_h^k(s, a)$ , then we have*

$$\bar{V}_h^k(s) \geq \min(H, b_t) \quad (18)$$

432 *Proof.* We have, for any  $(s, a, h, k) \in S \times A \times [H] \times [K]$ ,

$$\bar{Q}_h^k(s, a) = \alpha_t^0 H + \sum_{i=1}^t \alpha_t^i [\bar{V}_{h+1}^{k_i}(x_{h+1}^{k_i}) + b_i] \quad (19)$$

$$\geq \sum_{i=1}^t \alpha_t^i b_i \geq \sum_{i=1}^t \alpha_t^i b_t = b_t. \quad (20)$$

433 Thus,  $\bar{V}_h^k(s) \geq \min(H, \max_a \bar{Q}_h^k(s, a)) \geq \min(H, b_t)$ . ■

434 **Lemma 8.** *With probability at least  $1 - p$ , for any  $(s, a, h, k) \in S \times A \times [H] \times [K]$ , let  $t = N_h^k(s, a)$ ,*  
 435 *then we have*

$$\bar{Q}_h^k(s, a) \geq \sum_{i=1}^t \alpha_t^i [\mathbb{P}_h \bar{V}_{h+1}^{k_i}](s, a) \quad (21)$$

436 *Proof.* We have, for any  $(s, a, h, k) \in S \times A \times [H] \times [K]$ ,

$$Q_h^k(s, a) = \alpha_t^0 H + \sum_{i=1}^t \alpha_t^i [V_{h+1}^{k_i}(x_{h+1}^{k_i}) + b_i] \quad (22)$$

$$\geq \sum_{i=1}^t \alpha_t^i [\mathbb{P}_h \bar{V}_{h+1}^{k_i}(s, a) + (\hat{\mathbb{P}}_h^{k_i} - \mathbb{P}_h) \bar{V}_{h+1}^{k_i}(s, a) + b_i] \quad (23)$$

$$\stackrel{\text{w.p. } 1-p}{\geq} \sum_{i=1}^t \alpha_t^i [\mathbb{P}_h \bar{V}_{h+1}^{k_i}(s, a)] \quad (24)$$

437 The last inequality is by the same martingale bound as in the proof of Lemma 2. ■

438 Now, we are ready to prove Theorem 3.

439 **Proof of Theorem 3:** Let  $h^*, s^*, a^*$  be given, and denote  $t^* = N_{h^*}^K(s^*, a^*)$ ,  $b_t^* = c\sqrt{H^3 \iota / t^*}$ . Then,  
 440 by Lemma 7, we have

$$\bar{V}_{h^*}^K(s^*, a^*) \geq \min(H, b_{t^*}^*) \quad (25)$$

441 Now, by Lemma 8, we have that for any  $(s, a)$ ,

$$\bar{Q}_{h^*-1}^K(s, a) \geq \sum_{i=1}^t \alpha_t^i [\mathbb{P}_{h^*-1} \bar{V}_{h^*}^{k_i}](s, a) \quad (26)$$

$$\geq \sum_{i=1}^t \alpha_t^i P(s^* | s, a) \min(H, b_i) \quad (27)$$

$$= P(s^* | s, a) \min(H, b_t^*) \quad (28)$$

442 Thus, we have

$$\bar{V}_{h^*-1}(s) = \max_a \bar{Q}_{h^*-1}(s, a) \quad (29)$$

$$\geq \max_a P(s^*|s, a) \min(H, b_t^*) \quad (30)$$

$$= \delta_{h^*-1, h^*}(s, s^*) \min(H, b_t^*) \quad (31)$$

443 We now show by induction that for all  $h < h^*$ ,

$$\bar{V}_h(s) \geq \delta_{h, h^*}(s, s^*) \min(H, b_t^*) \quad (32)$$

444 We again use Lemma 8 to get

$$\bar{Q}_h(s, a) \geq \sum_{i=1}^t \alpha_t^i [\mathbb{P}_h \bar{V}_{h+1}^{k_i}](s, a) \quad (33)$$

$$\geq \sum_{i=1}^t \alpha_t^i \left[ \sum_{s' \in S} P(s'|s, a) \bar{V}_{h+1}^{k_i}(s') \right] \quad (34)$$

$$\geq \sum_{i=1}^t \alpha_t^i \left[ \sum_{s' \in S} P(s'|s, a) \delta_{h+1, h^*}(s', s^*) \min(H, b_t^*) \right] \quad (35)$$

$$= \sum_{s' \in S} P(s'|s, a) \delta_{h+1, h^*}(s', s^*) \min(H, b_t^*) \quad (36)$$

445 Then,

$$\bar{V}_h(s) = \max_a \sum_{s' \in S} P(s'|s, a) \delta_{h+1, h^*}(s', s^*) \min(H, b_t^*) \quad (37)$$

$$= \delta_{h, h^*}(s, s^*) \min(H, b_t^*), \quad (38)$$

446 where in the last equality, we use the Bellman optimality equation w.r.t.  $\delta$ , i.e.

447  $\delta_{h, h^*}(s, s^*) = \max_a \sum_{s' \in S} P(s'|s, a) \delta_{h+1, h^*}(s', s^*)$ . Therefore, we have established that

448  $\bar{V}_1(s) \geq \delta_{1, h^*}(s, s^*) \min(H, b_t^*)$ . This implies that

$$\sum_{k=1}^K \bar{V}_1^k(s_1) \geq K \delta(s^*) \min(H, b_t^*) \quad (39)$$

449 Furthermore, we know from the proof of Theorem 1 that

$$\sum_{k=1}^K \bar{V}_1^k(s_1) \leq O(\sqrt{H^5 S A K \iota}) \quad (40)$$

450 When  $K \geq \Omega\left(\frac{H^3 S A \iota}{\delta(s^*)}\right)$ ,  $\sum_{k=1}^K \bar{V}_1^k(s_1) \leq K \delta(s^*) H$ . Therefore, we have

$$K \delta(s^*) b_t^* = K \delta(s^*) c \sqrt{H^3 \iota / t^*} \leq O(\sqrt{H^5 S A K \iota}) \quad (41)$$

451 This gives us

$$t^* \geq O\left(\frac{K \delta(s^*)^2}{H^2 S A}\right). \quad (42)$$

452 This holds for any  $s^*, a^*, h^*$ , establishing the results. ■

453 **Proof of Theorem 4.** First, notice that for any given  $r_h(s, a, s')$  out of a set of size  $H S^2 A$ , by the  
454 proof of Theorem 1, we have

$$\sum_{k=1}^K (V_1^k - V_1^*)(s_1) \leq \sum_{k=1}^K \bar{V}_1^k \leq O\left(\sqrt{H^5 S A K}\right) \quad (43)$$

455 Define  $\tilde{V}_1^K = \frac{1}{K} \sum_{k=1}^K V_1^k(s_1)$ , then

$$0 \leq \tilde{V}_1^K - V_1^*(s_1) \leq O\left(\sqrt{\frac{H^5 S A \epsilon}{K}}\right) \leq \epsilon. \quad (44)$$

456 Now, let  $(h^*, s^*, a^*, s'^*)$  be given. Define reward functions  $R^{(1)}, R^{(2)}$  as

$$R_h^{(1)}(s, a, s') = \begin{cases} 1, & \text{if } h = h^*, s = s^*, a = a^*, s' = s'^* \\ 0, & \text{otherwise} \end{cases} \quad (45)$$

$$R_h^{(2)}(s, a, s') = \begin{cases} 1, & \text{if } h = h^*, s = s^* \\ 0, & \text{otherwise} \end{cases} \quad (46)$$

457 Then, we observe that the corresponding  $V_1^{*(1)} = \delta_{h^*}(s^*)P_{h^*}(s'^*|s^*, a^*)$  and  $V_1^{*(2)} = \delta_{h^*}(s^*)$ .

458 Now, define

$$\hat{P}(s'^*|s^*, a^*) = \frac{\tilde{V}_1^{K(1)}}{\tilde{V}_1^{K(2)}} \quad (47)$$

459 Next, we show that  $\|\hat{P}(s'^*|s^*, a^*) - P(s'^*|s^*, a^*)\|$  is small. In particular,

$$\hat{P}(s'^*|s^*, a^*) = \frac{\tilde{V}_1^{K(1)}}{\tilde{V}_1^{K(2)}} \quad (48)$$

$$\leq \frac{\delta_{h^*}(s^*)P_{h^*}(s'^*|s^*, a^*) + \epsilon}{\delta_{h^*}(s^*)} \quad (49)$$

$$= P(s'^*|s^*, a^*) + \frac{\epsilon}{\delta_{h^*}(s^*)}, \quad (50)$$

$$\hat{P}(s'^*|s^*, a^*) = \frac{\tilde{V}_1^{K(1)}}{\tilde{V}_1^{K(2)}} \quad (51)$$

$$\geq \frac{\delta_{h^*}(s^*)P_{h^*}(s'^*|s^*, a^*)}{\delta_{h^*}(s^*) + \epsilon} \quad (52)$$

$$\geq \frac{\delta_{h^*}(s^*)P_{h^*}(s'^*|s^*, a^*) - \epsilon}{\delta_{h^*}(s^*)} \quad (53)$$

$$= P(s'^*|s^*, a^*) - \frac{\epsilon}{\delta_{h^*}(s^*)}. \quad (54)$$

460 A union bound on all  $(h^*, s^*, a^*, s'^*) \in [H] \times S \times A \times S$  completes the proof. Notice that the  
461 sample complexity only changes by constant factor as  $\log(N) = \log(HS^2A) \leq 2\log(HSA)$ . ■

## 462 C Proof of Lower Bound

463 We based our construction on the classic lower-bound construction for multi-armed bandits. For a  
464 detailed introduction of the problem setting, please refer to [Mannor and Tsitsiklis, 2004]. We first  
465 introduce some bandit notation: let  $n$  be the number of arms,  $p \in [0, 1]^n$  represent the parameters  
466 of the Bernoulli distribution of rewards associated with each arm. We let  $T_\ell$  be the total number of  
467 times that arm  $\ell$  is pulled, and  $T = \sum_{\ell=1}^n T_\ell$  be the total number of arm pulls. We also let  $I$  be the  
468 arm that is selected at the end of the exploration phase.

469 **Lemma 9.** *There exists a  $p \in [0, 1]^n$ ,  $n \geq 2$  such that for any fixed number of episodes  $K$ , there  
470 exists  $N = O(2^K)$  reward functions, so that with probability at least 0.5, no RL algorithm can learn  
471 an  $\epsilon$ -optimal policy with  $\epsilon \leq 0.08$  for at least one reward function.*

472 *Proof.* We construct a bandit with two arms  $\ell = 1, 2$ . We consider two reward functions. The first  
473 reward function is  $p$  with  $p_1 = 0.1, p_2 = 0$  and the second reward function is  $q$  with  $q_1 = 0.1$ ,  
474  $q_2 = \text{Bernoulli}(0.5)$ . Thus, it is easy to see that the optimal arm corresponding to  $p$  and  $q$  are  $\ell = 1$   
475 and  $\ell = 2$  respectively. We assume among the  $N$  reward functions we need to learn,  $N - 1$  of them

are  $q$  and only one is  $p$ . Next, we show that no learner is able to distinguish whether the instantiated rewards are from  $p$  or  $q$ .

Let  $T_2$  be the number of episodes where arm 2 is taken in the  $K$  instantiated rewards. Then for each of the  $N - 1$  reward function  $q$ , it has probability  $0.5^{T_2}$  to generate the same instantiated rewards with  $r_1$ . Note that  $0.5^{T_2} \geq 0.5^K$ , so the probability that at least one of the  $q$  generate the same instantiated rewards as  $p$  is at least

$$1 - (1 - 0.5^K)^{N-1} \geq 1 - e^{-0.5^K(N-1)} \quad (55)$$

Let  $N = \lceil 1 + 2^K \ln 2 \rceil$ , then the probability that the rewards can be generated by one of the  $q$  is at least 0.5. Given such a reward configuration, let  $\hat{\pi} = (x, 1 - x)$  be the learned (stochastic) policy where  $x$  is the probability of choosing arm 1. Then for reward function  $q$ , the optimality gap is

$$V_2^* - V_2(\hat{\pi}) = 0.5 - 0.1x - (1 - x) * 0.5 = 0.4x, \quad (56)$$

while for reward function  $r_1$ , the optimality gap is

$$V_1^* - V_1(\hat{\pi}) = 0.1 - 0.1x. \quad (57)$$

One can see that regardless of  $p_1$ , one of the above two gaps will be large, and the minimum of  $\max(V_2^* - V_2(\hat{\pi}), V_1^* - V_1(\hat{\pi}))$  is achieved when  $p_1 = 0.2$ , and the minimum value is 0.08.

Therefore with probability at least 0.5, no RL algorithm can learn  $\varepsilon$ -optimal policy with  $\varepsilon = 0.08$ . ■

**Theorem 10.** *There exist some positive constant  $c_1, c_2, \varepsilon_0, \delta_0$ , such that for every  $n \geq 2, \varepsilon \in (0, \varepsilon_0)$ , and  $\delta \in (0, \delta_0)$ , and for every  $(\varepsilon, \delta)$ -correct policy on  $N$  tasks, there exists some  $p \in [0, 1]^n$  such that*

$$\mathbf{E}_p [T] \geq c_1 \frac{n}{\varepsilon^2} \log \frac{c_2 N}{\delta} \quad (58)$$

*Proof.* The proof largely mimic the original proof of Theorem 1 in [Mannor and Tsitsiklis, 2004], with the distinction in handling  $N$  tasks instead of 1. Consider a bandit problem with  $n + 1$  arms. We also consider a finite set of  $n + 1$  possible reward functions  $p$ , which we refer to as “hypotheses”. Under any one of the hypothesis, arm 0 has a Bernoulli reward with  $p_0 = (1 + \varepsilon)/2$ . Under one hypothesis, denoted  $H_0$ , all other arm has  $p_i = 1/2$ , which makes arm 0 the best arm. Furthermore, for  $\ell = 1, \dots, n$ , there is a hypothesis

$$H_\ell : p_0 = \frac{1 + \varepsilon}{2}, \quad p_\ell = \frac{1}{2} + \varepsilon, \quad p_i = \frac{1}{2}, \text{ for } i \neq 0, \ell. \quad (59)$$

which makes arm  $\ell$  the best arm. We define  $\varepsilon_0 = 1/8$  and  $\delta_0 = e^{-4}/8$ . From now on, we fix  $\varepsilon \in (0, \varepsilon_0), \delta \in (0, \delta_0), N \geq 1$  and a policy, which we assume to be  $(\varepsilon/2, \delta)$ -correct on  $N$  rewards. If  $H_0$  is true, the policy must have a probability at least  $1 - \delta$  of eventually stopping and selecting arm 0. If  $H_\ell$  is true, for some  $\ell \neq 0$ , the policy must have a probability at least  $1 - \delta$  of eventually stopping and selecting arm  $\ell$ . These further hold simultaneously for  $N$  hypotheses. We denote  $P_\ell^N(\cdot)$  as the probability of some event that happens simultaneously under  $N$   $H_\ell$  hypotheses.

We define  $t^*$  by

$$t^* = \frac{1}{c\varepsilon^2} \log \frac{N}{8\delta} = \frac{1}{c\varepsilon^2} \log \frac{N}{\theta} \quad (60)$$

where  $\theta = 8\delta$  and  $c$  is an absolute constant we will specify later. Note that  $\theta < e^{-4}$  and  $\varepsilon \leq 1/4$ .

We assume by contradiction that  $\mathbf{E} [T_1] \leq t^*$ . We will eventually show that under this assumption, the probability of selecting  $H_0$  under one of  $N$   $H_1$  exceeds  $\delta$ , thus violates  $(\varepsilon/2, \delta)$ -correctness.

We now introduce some special events A, B and C. We define

$$A = \{T_1 \leq 4t^*\} \quad (61)$$

$$B = \{I = 0, \text{ i.e. the policy eventually pick arm 0}\} \quad (62)$$

$$C = \left\{ \max_{1 \leq t \leq 4t^*} |K_t - \frac{1}{2}t| < \sqrt{t^* \log(N/\theta)} \right\} \quad (63)$$

where  $K_t$  is the number of getting reward 1 if the first arm is pulled  $t$  times. Similar to the original proof [Mannor and Tsitsiklis, 2004], we have the following lemmas.

510 **Lemma 11.**  $P_0^N(A) = P_0(A) > 3/4$ , where  $P_0^N(C)$  denotes the probability of event  $B$  under all of  
 511  $N$  hypothesis  $H_0$ .

512 This is directly due to the definition of  $A$  that is independent of rewards and the use of Markov  
 513 inequality.

514 **Lemma 12.**  $P_0^N(B) > 3/4$ .

515 This is due to  $\delta < e^{-4}/8 < 1/4$ .

516 **Lemma 13.**  $P_0^N(C) > 3/4$ .

517 This is due to the observation that  $K_t - t/2$  is a martingale, and by applying Kolmogorov's inequality.

518 **Lemma 14.** If  $0 \leq x \leq 1$  and  $y \geq 0$ , then

$$(1 - x)^y \geq e^{-dxy} \quad (64)$$

519 where  $d = 1.78$

520 This is straightforward arithmetics. Please refer to the original proof in [Mannor and Tsitsiklis, 2004]  
 521 for the detailed proofs of the lemmas. Let  $S = A \cap B \cap C$ , then we have  $P_0^N(S) > 1/4$ . Now we are  
 522 ready to prove our main results. Let  $W$  be the history of the process (the number of arm pulls for each  
 523 arm in the exploration phase, and the sampled rewards in the policy-optimization phase). We define  
 524  $L_\ell(W)$  to be the likelihood of a history  $W$  under reward function  $\ell$ . We denote  $K$  be a shorthand  
 525 notation for  $K_{T_1}$ , the number of reward 1 instantiated on arm  $\ell = 1$ . Observe that, given the history  
 526 up to time  $t - 1$ , the arm choice at time  $t$  has the same probability distribution under either hypothesis  
 527  $H_0$  and  $H_1$ ; similarly, the arm reward at time  $t$  has the same probability distribution, under either  
 528 hypothesis, unless the chosen arm was arm 1. For this reason, the likelihood ratio  $L_1(W)/L_0(W)$  is  
 529 given by

$$\frac{L_1(W)}{L_0(W)} = \frac{(\frac{1}{2} + \varepsilon)^K (\frac{1}{2} - \varepsilon)^{T_1 - K}}{(\frac{1}{2})^{T_1}} \quad (65)$$

$$= (1 - 4\varepsilon^2)^K (1 - 2\varepsilon)^{T_1 - 2K} \quad (66)$$

530 Let  $T_1^N(W)$  be the likelihood that  $W$  appears under one of  $N$  hypotheses  $H_1$ . Since the instantiation  
 531 of rewards under each hypothesis is completely independent from one another, we have

$$L_1^N(W) = 1 - (1 - L_1(W))^N \quad (67)$$

$$\geq 1 - \frac{1}{1 + L_1(W)N} \quad (68)$$

$$= \frac{L_1(W)N}{1 + L_1(W)N} \quad (69)$$

532 By lemma 9, we have that in order for the policy to be  $\varepsilon, \delta$ -correct,  $T_1 \geq \log_2(N)$ . Thus, we have

$$L_1(W) \leq (\frac{1}{2} + \varepsilon)^K (\frac{1}{2} - \varepsilon)^{T_1 - K} \quad (70)$$

$$\leq (\frac{1}{2})^{T_1} \quad (71)$$

$$\leq \frac{1}{N} \quad (72)$$

533 We then have

$$\frac{L_1^N(W)}{L_0(W)} = \frac{L_1(W)N}{1 + L_1(W)N} \frac{1}{L_0(W)} \quad (73)$$

$$\geq \frac{N}{2} \frac{L_1(W)}{L_0(W)} \quad (74)$$

$$= \frac{N}{2} (1 - 4\varepsilon^2)^K (1 - 2\varepsilon)^{T_1 - 2K} \quad (75)$$

534 If event  $S$  occurred, then  $A$  occurred, and we have  $K \leq T_1 \leq 4t^*$ , so that

$$(1 - 4\epsilon^2)^K \geq (1 - 4\epsilon^2)^{4t^*} = (1 - 4\epsilon^2)^{\frac{1}{c\epsilon^2} \log \frac{N}{\theta}} \quad (76)$$

$$\geq e^{-(16d/c) \log(N/\theta)} \quad (77)$$

$$= (\theta/N)^{16d/c} \quad (78)$$

535 We have used here Lemma 14, which applies because  $4\epsilon^2 < 4/4^2 < 1/\sqrt{2}$ . Similarly, if event  $S$  has  
536 occurred, then  $A \cap C$  has occurred, which implies

$$T_1 - K \leq 2\sqrt{t^* \log(N/\theta)} = (2/\epsilon\sqrt{c}) \log(N/\theta). \quad (79)$$

537 Therefore,

$$(1 - 2\epsilon)^{T_1 - 2K} \geq (1 - 2\epsilon)^{(2/\epsilon\sqrt{c}) \log(N/\theta)} \quad (80)$$

$$\geq e^{-(4d/\sqrt{c}) \log(N/\theta)} \quad (81)$$

$$= (\theta/N)^{4d/\sqrt{c}} \quad (82)$$

538 Substituting the above into the main equation, we obtain

$$\frac{L_1^N(W)}{L_0(W)} \geq \frac{N}{2} (\theta/N)^{(16d/c) + 4d/\sqrt{c}} \quad (83)$$

539 By picking  $c$  large enough ( $c = 100$  suffices), we obtain that  $\frac{L_1^N(W)}{L_0(W)} \geq \theta/2 \geq 4\delta$  whenever the event  
540  $S$  occurs. More precisely, we have

$$\frac{L_1^N(W)}{L_0(W)} \mathbb{1}[S] \geq 4\delta \mathbb{1}[S] \quad (84)$$

541 where  $\mathbb{1}[S]$  is the indicator function of the event  $S$ . Then,

$$P_1^N(B) \geq P_1^N(S) = \mathbb{E}_1^N[\mathbb{1}[S]] = \mathbb{E}_0^N\left[\frac{L_1^N(W)}{L_0(W)} \mathbb{1}[S]\right] \geq \mathbb{E}_0^N[4\delta \mathbb{1}[S]] = 4\delta P_0^N(S) > \delta. \quad (85)$$

542 where we used the fact that  $P_0^N(S) > 1/4$ . This contradicts the assumption that the policy is  
543  $(\epsilon/2, \delta)$ -correct. Similarly, we must have  $\mathbf{E}[T_\ell] > t^*$ , for all arms  $\ell > 0$ . Therefore, if we have an  
544  $(\epsilon, \delta)$ -correct policy, we must have  $\mathbf{E}[T] > (n/(4c\epsilon^2)) \log(N/8\delta)$ , which is of the desired form.

545 ■

546 Now we are ready to prove theorem 5.

547 **Proof of theorem 5.** We consider an MDP  $M$  where the transition is defined as  $P_h(s'|s, a) = 1/S$   
548 for all  $(h, s, a, s')$  and is **known** to the learner. Since the action has no control over the next-  
549 state, this is equivalent to a collection of  $SH$  multi-armed bandits. Due to the uniform transition,  
550  $P_h^\pi(s) = 1/S$  for any  $\pi, s, h$ , and so finding the  $\epsilon$ -optimal policy amounts to finding an  $\epsilon_{s,h}$ -optimal  
551 policy for each bandit  $(s, h)$ , such that  $\sum_{s,h} \epsilon_{s,h} = S\epsilon$ . Theorem 10 implies that it takes at least  
552  $\Omega(A \log(N/p)/\epsilon_{s,h}^2)$  visits to a bandit  $s, h$  to find an  $\epsilon_{s,h}$ -optimal action simultaneously for each  
553 of  $N$  reward functions with probability at least  $1 - p$ . It follows that the total number of samples  
554 required  $\Omega(\sum_{s,h} A \log(N/p)/\epsilon_{s,h}^2)$  is minimized when  $\epsilon_{s,h} = \epsilon/H$  for all  $(s, h)$ , which gives a total  
555 of at least  $\Omega(H^3 S A \log(N/p)/\epsilon^2)$  samples, which translates to at least  $\Omega(H^2 S A \log(N/p)/\epsilon^2)$   
556 episodes. ■

## 557 D Proof of $N$ -independent upper bound of UCBZERO in the Reward-free 558 Setting

559 **Proof of Theorem 6.** Fixing the transition kernel, we consider dividing all possible MDPs into a  
560 set of equivalence classes based on different reward patterns. Specifically, given any  $M \in \mathbb{Z}^+$ , we  
561 split the support of reward  $[0, 1]$  into  $M$  segments,  $I_i = [\frac{i-1}{M}, \frac{i}{M}]$ ,  $\forall 1 \leq i \leq M$ . For any MDP,

the reward function  $r_h(s, a)$  depends only on state  $s$  and action  $a$ , and for each  $(s, a)$  pair, the corresponding reward must lie in one of the  $M$  segments, thus there are  $M^{|S| \times |A|}$  different patterns of reward functions for each step  $h$ , characterized by a matrix  $\Phi_h \in [M]^{|S| \times |A|}$ , where each entry  $\Phi_h(i, j) \in [M]$  is the segment that  $r_h(i, j)$  lies in. Given that we have  $H$  steps, in total we will have  $M^{|S| \times |A| \times H}$  different reward patterns, denoted as  $\Phi = \prod_{h=1}^H \Phi_h$ . For each  $\Phi$ , we next show that learning any single reward function  $r \in \Phi$  is enough to cover all other reward functions in  $\Phi$ . Specifically, assume we have learned a near-optimal policy  $\pi_r$  that satisfies

$$V_r^*(s_1) - V_r^{\pi_r}(s_1) < \varepsilon, \quad (86)$$

where subscript  $r$  means the value function under reward function  $r$  and  $V_r^{\pi_r}$  is the value function of the learned policy. Then for any other  $r' \in \Phi$  different from  $r$ , we have

$$V_{r'}^* - V_{r'}^{\pi_r} = V_{r'}^* - V_r^* + V_r^* - V_r^{\pi_r} + V_r^{\pi_r} - V_{r'}^{\pi_r}. \quad (87)$$

Note that

$$\begin{aligned} V_{r'}^* - V_r^* &= \max_{\pi} \mathbf{E}_{\pi} \left[ \sum_{h=1}^H r'_h(s_h, a_h) \right] - \max_{\pi} \mathbf{E}_{\pi} \left[ \sum_{h=1}^H r_h(s_h, a_h) \right] \\ &\leq \max_{\pi} \mathbf{E}_{\pi} \left[ \sum_{h=1}^H r'_h(s_h, a_h) - r_h(s_h, a_h) \right] \leq \frac{H}{M}, \end{aligned} \quad (88)$$

where the last inequality is due to  $r'_h$  and  $r_h$  lie in the same segment for all  $h$ . Same result holds for  $V_r^{\pi_r} - V_{r'}^{\pi_r}$ . Let  $M = \frac{H}{\varepsilon}$ . Then plug (88) back to (87), and also remember that  $V_r^*(s_1) - V_r^{\pi_r}(s_1) < \varepsilon$ , thus we have

$$V_{r'}^* - V_{r'}^{\pi_r} < \frac{H}{M} + \varepsilon + \frac{H}{M} = \frac{2H}{M} + \varepsilon = 3\varepsilon, \quad (89)$$

which shows that the policy learned on reward function  $r$  is also near-optimal for other reward functions in the same equivalence class. Given that, it suffices for our UCBZero to successfully learn a total of  $M^{|S| \times |A| \times H}$  reward functions in order to cover all possible MDPs. Then simply applying the conclusion in Theorem 1 concludes the proof. ■
